# Supplementary material for: LEASGD: an Efficient and Privacy-Preserving Decentralized Algorithm for Distributed Learning
Source: arXiv:1811.11124 source file (2018-11-27)
Supplement: Supplementary file 1 [file 9_supplementary_material.tex]

\section{Supplementary Material}
\subsection{Algorithm 1}
\begin{algorithm}[]
\caption{Synchronous Follower Elastic Averaging Stochastic Gradient Descent Gradient Descent}
\begin{algorithmic}[1]
\STATE {\textbf{Require:}} initial parameter vectors $w_0^i$, the number of workers $m$, the number of followers $L$, categorization interval $k$, communication interval $\tau$, elastic factor $\rho$, learning rate $\eta$
\STATE \FOR{\textbf{$iteration t=1,2,......,T$}}
\STATE \IF {\textbf{$t\ mod\ k\tau\ is\ 0$}}
\STATE \IF {\textbf{$t\ =\ 0$}}
\STATE randomly select $L$ followers $l_1,......,l_L$
\STATE \ELSE 
\STATE sort the loss function value and categorize $L$ followers
\STATE $\ \ \ \ {l_1,......,l_L}= \mathop{argmaxL}\limits_{i=1,...,m}f^i_t(\omega^i)$
\ENDIF
\ENDIF
\STATE \IF{$t\ mod\ \tau\ is\ 0$}
\STATE \FOR{\textbf{followers:}$i\in \{l_1,......,l_L\}$}
\STATE  local SGD updating
\ENDFOR
\STATE \FOR{\textbf{ followers:$i\notin \{l_1,......,l_L\}$}}
\STATE randomly select a follower $f$ from follower pool
\STATE transmit parameter vectors with $f$ and do elastic updating
\ENDFOR
\STATE \ELSE
\STATE \FOR{\textbf{all workers: }$i\in \{1,......,m\}$}
\STATE  local SGD updating
\ENDFOR
\ENDIF
\ENDFOR
\end{algorithmic}
\end{algorithm}

\subsection{Detail Proof of Proposition 1}
Before we show the result of the convergence rate, we first introduce some assumptions held in the analysis.
\newtheorem{assumption}{Assumption}%[section]
\begin{assumption}\label{ass:ass1}

These assumptions are held throughout the analysis:\\
1. \textbf{i.i.d. assumption}: We divide our system into several sub-systems with only 1 follower and $p$ leaders. And all the variables in these sub-systems are i.i.d.\\
2. \textbf{Correct categorization}: Assume that since the categorization step in Algorithm 1 is implemented, the identity of all workers will not change until the next categorization\\
3. \textbf{Bounded stochastic gradient}: Assume that the variance of all the local gradients is bounded for any $w$ for any workers from ${1,...,m}$ and input $x^i_t$. There exist constant $\sigma_1$ such that \begin{equation}
    \label{bound_gradient}
    \begin{split}
        E[g^i_t-\bigtriangledown f(w^i_t)]=0\ and\\
        E[\parallel g^i_t-\bigtriangledown f(w^i_t)\parallel^2]\le\sigma_1^2
    \end{split}
\end{equation}
4. \textbf{Strongly convex condition}: We only discuss about the strongly-convex case in the analysis. Correspondlingly, there exists $0<\mu\le L$ for all the loss functions:

\begin{equation}
    \label{regularized_function}
    %\begin{split}
        f^i_{t}(w^i)=l(w^i_t,x^i_t,y^i_t)+\lambda\parallel w^i\parallel_2
    %\end{split}
\end{equation}

and we can rewrite it to:

\vspace{-7mm}

\begin{equation}
    \label{strongly_convex}
    \begin{split}
        \mu \parallel w_i-w_j \parallel ^2 \le \langle\bigtriangledown f(w_i),\bigtriangledown f(w_j)\rangle\le L\parallel w_i-w_j \parallel ^2
    \end{split}
\end{equation}
\end{assumption}

\vspace{-6mm}

We define that
\begin{equation}
    \label{d_t}
    \begin{split}
        d_t=\frac{E\sum_{i=1}^{p}\parallel w^i_t-w^*\parallel^2+E\parallel w^f_t-w^*\parallel^2}{p+1}
    \end{split}
\end{equation}

\vspace{-3mm}

and under Assumption \ref{ass:ass1}, we can obtain the result of convergence rate of $d_t$ in Algorithm 1

We first provide the proof of convergence rate of Algorithm 1 under a strongly-convex case. In the analysis, we mainly focused on the average square of the distance between all workers to the optimum, that is $d_t$ shown in the proposition. We draw the ideas from the convergence analysis of EASGD under a strongly-convex case \cite{zhang2015deep} but further specify it to our algorithm. Under the first assumption in Assumption \ref{ass:ass1}, we simplify our system by dividing it into several subsystems and each includes only 1 follower and $p$ leaders. We assume that the convergence rate of each subsystem is the same as that of the whole system. 

To obtain this convergence rate, we will need following theorem.
\begin{mytheo}
Let $y_t= \frac{1}{p}\sum_{i=1}^{p} w^i_t$, $a_t=E\parallel y_t-w^*\parallel^2$, $b_t=\frac{1}{p}\sum_{i=1}^{p}E\parallel w^i_t-w^*\parallel^2$, $c_t=E\parallel w^f_t-w^*\parallel^2$, $\alpha=\eta\rho$, $\beta=p\alpha$,$\gamma=2\eta\frac{\mu L}{\mu+L}$. If $0\le\eta\le\frac{2(1-\beta)}{\mu+L}$,$0\le\alpha<1$,$0\le\beta<1$, then
\begin{align}
    b_{t+1}\le(1-\gamma-\alpha)b_t+\alpha c_t+\eta^2\sigma_1^2\\
    c_{t+1}\le(1-\gamma-\beta)c_t+\beta a_t+\eta^2\sigma_1^2
\end{align}
\end{mytheo}

\emph{Proof}
Under the third assumption of Assumption \ref{ass:ass1}, the noisy gradient $g_t^i$ of all the workers can be rewritten as $g_t^i=\bigtriangledown f(w^i_t)+\xi_t^i$ in which $E[\xi_t^i]=0$ and $E\parallel \xi_t^i\parallel^2<\sigma_1^2$. Then the updating rules of Algorithm 1 could be written as
\begin{align}
    w^i_{t+1}=w^i_t-\eta g_t^i-\alpha(w_t^i-w_t^f)\\
    w^f_{t+1}=w^f_t-\eta g_t^f-\beta(w_t^f-y_t)
\end{align}
From equation (3), we have 
\begin{equation}
    \begin{split}
        \parallel w_{t+1}^i-w^*\parallel^2= \parallel w_t-w^*\parallel^2+\eta^2\parallel g_t^i\parallel^2+\alpha^2\parallel w^i_t-w^f_t \parallel^2\\
        -2\eta\langle g_t^i,w^i_t-w^*\rangle-2\alpha \langle w_t^i-w^f_t,w^i_t-w^*\rangle\\+2\eta\alpha\langle g_t^i,w^i_t-w^f_t\rangle
    \end{split}
\end{equation}
By the cosine rule($2\langle a-b,c-d\rangle=\parallel a-d \parallel^2-\parallel a-c \parallel^2+\parallel c-b \parallel^2-\parallel b-d \parallel^2$), we have
\begin{equation}
    \begin{split}
        2\langle w_t^i-w^f_t,w^i_t-w^*\rangle=\parallel w_t^i-w^* \parallel^2+\parallel w^i_t-w^f_t \parallel^2\\
        -\parallel w^f_t-w^* \parallel^2
    \end{split}
\end{equation}

By Cauchy-Schwarz inequality, we have
\begin{equation}
    \begin{split}
        \langle \bigtriangledown f(w^i_t),w^i_t-w^f_t\rangle\le\parallel \bigtriangledown f(w^i_t)\parallel\parallel w^i_t-w^f_t\parallel
    \end{split}
\end{equation}
In the strongly-convex case, we use following theorem of strongly-convex function \cite{nesterov2004introductory}
\begin{equation}
    \begin{split}
        \langle \bigtriangledown F(x)-\bigtriangledown F(y),x-y\rangle\ge\frac{\mu L}{\mu+L}\parallel x-y\parallel^2\\
        +\frac{1}{\mu+L}\parallel \bigtriangledown F(x)-\bigtriangledown F(y)\parallel^2
    \end{split}
\end{equation}
Since $\bigtriangledown f(w^*)=0$, we have
\begin{equation}
    \begin{split}
        \langle \bigtriangledown f(w^i_t),w^i_t-w^*\rangle \ge \frac{\mu L}{\mu+L}\parallel w^i_t-w^*\parallel^2+\frac{1}{\mu+L}\parallel g_t^i\parallel^2
    \end{split}
\end{equation}
Using (5),(6),(7),(9), we thus have
\begin{equation}
    \begin{split}
        \parallel w_{t+1}^i-w^*\parallel^2\le \parallel w_t-w^*\parallel^2+\eta^2\parallel \bigtriangledown f(w^i_t)+\xi^i_t\parallel^2+\alpha^2\parallel w^i_t-w^f_t \parallel^2\\
        -2\eta(\frac{\mu L}{\mu+L}\parallel w^i_t-w^*\parallel^2+\frac{1}{\mu+L}\parallel \bigtriangledown f(w_t^i)\parallel^2)-2\eta\langle \xi^i_t,w^i_t-w^*\rangle\\
        -\alpha(\parallel w_t^i-w^* \parallel^2+\parallel w^i_t-w^f_t \parallel^2-\parallel w^f_t-w^* \parallel^2)\\
        +2\eta\alpha\parallel \bigtriangledown f(w^i_t)\parallel\parallel w^i_t-w^f_t\parallel+2\eta\alpha\langle \xi^i_t,w^i_t-w^f_t\rangle
    \end{split}
\end{equation}
With $0\le\alpha<1$, we bound the term 
\begin{equation}
    \begin{split}
        \alpha^2\parallel w^i_t-w^f_t \parallel^2-\alpha\parallel w^i_t-w^f_t \parallel^2+2\eta\alpha\parallel \bigtriangledown f(w^i_t)\parallel\parallel w^i_t-w^f_t\parallel\\
=\alpha(1-\alpha)\parallel w^i_t-w^f_t \parallel^2+2\eta\alpha\parallel \bigtriangledown f(w^i_t)\parallel\parallel w^i_t-w^f_t\parallel\\
\le\frac{\eta^2\alpha}{1-\alpha}\parallel \bigtriangledown f(w^i_t)\parallel^2
    \end{split}
\end{equation}
by applying $-ax^2+bx\le\frac{b^2}{4a}$ with $x=\parallel w^i_t-w^f_t \parallel^2$. 
Thus, we obtain
\begin{equation}
    \begin{split}
        \parallel w_{t+1}-w^*\parallel^2\le (1-2\eta\frac{\mu L}{\mu+L}-\alpha)\parallel w_t^i-w^*\parallel^2\\
        +(\eta^2+\frac{\eta^2\alpha}{1-\alpha}-\frac{2\eta}{\mu+L})\parallel \bigtriangledown f(w^i_t)\parallel^2+2\eta^2\langle \bigtriangledown f(w^i_t),\xi^i_t\rangle\\
        -2\eta\langle \xi^i_t,w^i_t-w^*\rangle+2\eta\alpha\langle \xi^i_t,w^i_t-w^f_t\rangle
        +\eta^2\parallel \xi^i_t\parallel^2
        \\+\alpha\parallel w^f_t-w^*\parallel^2
    \end{split}
\end{equation}
Given that $E[\xi_t^i]=0$ and $E\parallel \xi_t^i\parallel^2<\sigma_1^2$ and if $\eta$ satisfies $\eta^2+\frac{\eta^2\alpha}{1-\alpha}-\frac{2\eta}{\mu+L}\le0$, then we have
\begin{equation}
    \begin{split}
        E\parallel w_{t+1}-w^*\parallel^2\le(1-2\eta\frac{\mu L}{\mu+L}-\alpha)E\parallel w_t^i-w^*\parallel^2\\
        +\eta^2\sigma^2_1+\alpha\parallel w^f_t-w^*\parallel^2
    \end{split}
\end{equation}
This concludes the proof of (1).
We discover that equation (4) is very similar to the equation (3). If we change
\begin{align}
    w^i_t\to w^i_f\\
    g^i_t\to g^f_t\\
    w^f_t\to y_t\\
    \alpha\to\beta
\end{align}
(3) can be transformed to (4). Thus, we obtain the (2) in the similar way as (1).
Next, we give the proof of Proposition 1 based on (1) and (2).

\begin{mypro}{(Convergence rate of Algorithm 1)}
If $0\le\eta\le\frac{2(1-\beta)}{\mu+L}$,$0\le\alpha<1$,$0\le\beta=p\alpha<1$, then we obtain the convergence of $d_t$\\
\begin{equation}\label{eq:rate}
    \begin{split}
        d_{t}\le h^t d_0+(c_0-\frac{\eta^2\sigma_1^2}{\gamma})(1-\gamma)^t(1-(\frac{p}{p+1})^t)+\eta^2\sigma_1^2\frac{1-h^t}{\gamma},\\
        where\  0<h=\frac{p(1-\gamma)}{p+1}<1,k=\frac{1-\gamma}{p+1},\gamma=2\eta\frac{\mu L}{\mu+L}\\
        and\ c_0=\mathop{max}\limits_{i=1,...,p,f}\parallel w^i_0-w^*\parallel^2
    \end{split}
\end{equation}
\end{mypro}

\emph{Proof} From the sorting rule and the Assumption 5.1(2), we can easily obtain the inequality relation of $a_t$,$b_t$,$c_t$ and $d_t$
\begin{align}
    a_t\le d_t\le c_t\\
    and\ b_t\le d_t\le c_t
\end{align}
Applying (19) in (2), we have
\begin{equation}
    \begin{split}
         c_{t+1}\le(1-\gamma-\beta)c_t+\beta a_t+\eta^2\sigma_1^2\\
         \le(1-\gamma-\beta)c_t+\beta c_t+\eta^2\sigma_1^2\\
         =(1-\gamma)c_t+\eta^2\sigma_1^2
    \end{split}
\end{equation}
Through iterating this inequality with $t$, we have
\begin{equation}
    \begin{split}
         c_t\le(1-\gamma)^tc_0+\eta^2\sigma_1^2[1+(1-\gamma)+......+(1-\gamma)^t]\\
         =(1-\gamma)^tc_0+\eta^2\sigma_1^2\frac{1-(1-\gamma)^t}{\gamma}
    \end{split}
\end{equation}
Noting that $d_t=\frac{pb_t+c_t}{p+1}$ and use the (1),(2), we have
\begin{equation}
    \begin{split}
        d_t=\frac{pb_t+c_t}{p+1}\\
        \le\frac{p}{p+1}[(1-\gamma-\alpha)b_{t-1}+\alpha c_{t-1}+\eta^2\sigma_1^2]\\
        +\frac{1}{p+1}[\beta a_{t-1}+(1-\gamma-\alpha)c_{t-1}+\eta^2\sigma_1^2]\\
        =\frac{p(1-\gamma)}{p+1}d_{t-1}+\frac{1-\gamma}{p+1}c_{t-1}+\eta^2\sigma_1^2\\
        =h d_{t-1}+kc_{t-1}+\eta^2\sigma_1^2
    \end{split}
\end{equation}
Applying (20) in (21), we have
\begin{equation}
    \begin{split}
        d_t\le h d_{t-1}+k[(1-\gamma)^{t-1}c_0+\eta^2\sigma_1^2\frac{1-(1-\gamma)^{t-1}}{\gamma}]+\eta^2\sigma_1^2\\
        =h d_{t-1}+k(c_0-\frac{\eta^2\sigma_1^2}{\gamma})(1-\gamma)^{t-1}+(1+\frac{k}{\gamma})\eta^2\sigma_1^2
    \end{split}
\end{equation}
Through iterating this inequality with $t$, we have
\begin{equation}
    \begin{split}
        d_t\le h^t d_0+k(c_0-\frac{\eta^2\sigma_1^2}{\gamma})[(1-\gamma)^{t-1}+h(1-\gamma)^{t-2}+......+h^{t-1}]\\
        +(1+\frac{k}{\gamma})\eta^2\sigma_1^2[1+h+......+h^{t-1}]\\
        = h^t d_0+k(c_0-\frac{\eta^2\sigma_1^2}{\gamma})\frac{(1-\gamma)^t-h^t}{1-\gamma-h}+(1+\frac{k}{\gamma})\eta^2\sigma_1^2\frac{1-h^t}{1-h}
    \end{split}
\end{equation}
To simplify (25), we note that
\begin{align}
    k+h=1-\gamma\\
    \frac{1+\frac{k}{\gamma}}{1-h}=\frac{1+\frac{\frac{1-\gamma}{p+1}}{\gamma}}{1-\frac{p(1-\gamma)}{p+1}}\\
    =\frac{p+1+\frac{1-\gamma}{\gamma}}{p+1-p(1-\gamma)}\\
    =\frac{p+\frac{1}{\gamma}}{1+p\gamma}\\
    =\frac{1}{\gamma}
\end{align}
Hence, (25) can be rewriten as
\begin{equation}
    \begin{split}
         d_t\le h^t d_0+(c_0-\frac{\eta^2\sigma_1^2}{\gamma})[(1-\gamma)^t-h^t]+\frac{1}{\gamma}\eta^2\sigma_1^2(1-h^t)\\
         =h^t d_0+(c_0-\frac{\eta^2\sigma_1^2}{\gamma})(1-\gamma)^t(1-(\frac{p}{p+1})^t)+\eta^2\sigma_1^2\frac{1-h^t}{\gamma}
    \end{split}
\end{equation}
This concludes the proof.

\subsection{Comparison of convergence rate of LEASGD and DPSGD in the strongly-convex case}
We provide a proof to demonstrate the convergence rate of our LEASGD algorithm faster than that of DPSGD when $t \to \infty$.

\emph{Proof} Remember the two convergence rate of both algorithms is $O(1/[(p+1)t])$ and $O(h^t)$ respectively for DPSGD and LEASGD in the strongly-convex case. 
By dividing one with another, we have
\begin{equation}
    \begin{split}
        \frac{O(1/(p+1)t)}{O(h^t)}\\
        ={\lim_{t \to +\infty}} \frac{1/[(p+1)t]}{h^t}\\
        ={\lim_{t \to +\infty}} \frac{(1/h)^t}{(p+1)t}
    \end{split}
\end{equation}
Using L'Hospital's Rule and note $1/h>1$, we thus have
\begin{equation}
    \begin{split}
        {\lim_{t \to +\infty}} \frac{(1/h)^t}{(p+1)t}\\
        ={\lim_{t \to +\infty}} \frac{[(1/h)^t]'}{[(p+1)t]'}\\
        ={\lim_{t \to +\infty}} \frac{(1/h)^t ln(1/h)}{p+1}\\
        =\infty
    \end{split}
\end{equation}
This concludes proof.
